# Supplementary material for: Automatic Zig-Zag sampling in practice
Source: arXiv:2206.11410 ancillary file (2022-09-02)
Supplement: Supplementary file 1 [file SI_CSRautomaticZZ.pdf]

# Supplement to *Automatic Zig-Zag sampling in practice.*

A. Corbella, S. E. F. Spencer, G. O. Roberts

June 2022

**Abstract**

This report is the supplement to the paper *Automatic Zig-Zag sampling in practice.* It provides background and specifics for the methods and the result presented. Specifically, it includes a description of the tuning of the Hamiltonian Monte Carlo (HMC) algorithm; the computation of the batch-means estimates of the Effective Sample Size (ESS) for continuous-time Markov chain Monte Carlos (MCMCs) and the choice of batch number; comprehensive results from the simulation study to assess the performance of the Automatic Zig-Zag algorithm; and lastly some background for the extreme-value methods used in the automatic subsampling.

## S1 Tuning of the HMC algorithm

The Automatic Zig-Zag sampling is benchmarked against canonical HMC. The canonical HMC algorithm, described in details in Neal et al., 2011, is summarised in the pseudocode of Algorithm 1.

The tuning of the HMC algorithm is well known to be a complicated problem (see, e.g. Sherlock, Urbas, and Ludkin, 2021). Even in the case considered here of the Canonical HMC, where the mass matrix is fixed and given ($\mathcal{M} = \mathbb{I}_d$), it is hard to find the adequate total integration time $L\varepsilon$, number of steps $L$, and step length $\varepsilon$.
In our case we choose to proceed as follows:

1. Set the number of steps to a fixed high value (e.g. for the bivariate normal $L = 10$ would suffice);
2. Tune the total integration time $L\varepsilon$ by running several chains with decreasing values of $L\varepsilon$ and choosing the first value for which we have very low autocorrelation and no antithetic behaviour in the fastest-moving component;
3. Inspect graphically the leapfrog trajectories of the proposed values in the first steps of the algorithm and check for anomalies;
4. Tune the number of leapfrog steps $L$ by running several chains with increasing values of $L$ and selecting the first value for which we have a desired average acceptance rate of 0.69 (from Neal et al., 2011).

**Result:** $N$ samples: $\{x_n\}_{n=1}^{N}$

**Input:** $x_0$: starting point of the algorithm; $N$: total number of samples desired; $\varepsilon$ stepsize of the leapfrog method; $L$: number of steps for the leapfrog method; $U(\cdot)$ and $\nabla U(\cdot)$: functions to compute the negative log target desnity and its gradient.

$q = x_0$ # set initial position
**for** $n = 1, 2, \ldots N$ **do**
  $q = x_{n-1}$ # set starting position
  $p \sim \mathcal{N}(0; \mathbb{I}_d)$ # set starting momentum
  $p^* = p$ ; $q^* = q$ # initialize proposed momentum and position
  $p^* = p^* - \frac{\varepsilon}{2} \nabla U(q^*)$ # half step for the momentum
  **for** $l = 1, 2, \ldots L - 1$ **do**
    $q^* = q^* + \varepsilon p^*$ # full step for the position
    $p^* = p^* - \varepsilon \nabla U(q^*)$ # full step for the momentum
  **end**
  $q^* = q^* + \varepsilon p^*$ # $L$th full step for the position
  $p^* = p^* - \frac{\varepsilon}{2} \nabla U(q^*)$ # half step for the momentum
  $p^* = -p^*$ # negate the momentum
  $V = U(q)$ # current potential
  $V^* = U(q^*)$ # proposed potential
  $K = \sum_{i=1}^{d} (p_i)^2$ # current kinetic energy
  $K^* = \sum_{i=1}^{d} (p_i^*)^2$ # proposed kinetic energy
  $u \sim \mathrm{Ber} \exp\{V - V^* + K - K^*\}$ # accept/reject Metropolis step
  **if** $u = 1$ **then**
    $x_n = q^*$ # retain the proposed position
  **else**
    $x_n = q^*$ # retain the starting position
  **end**
**end**

**Algorithm 1:** Pseudocode of the Canonical[1] HMC algorithm.

Figure S1 illustrates how Step 2 and Step 3 are performed on a bivariate isotropic Normal distribution: when the total integration time $L\varepsilon$ is too small the chain struggles to explore the space, and when it is too large it shows strong inverse autocorrelation and antithetic behaviour.

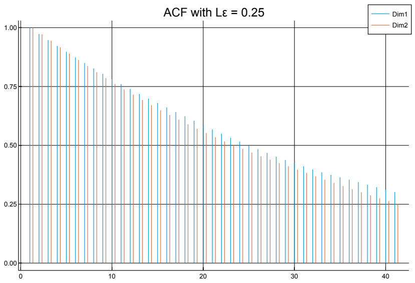


(a)

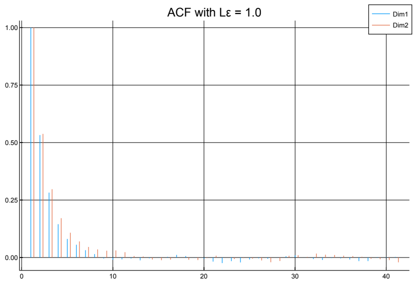


(b)

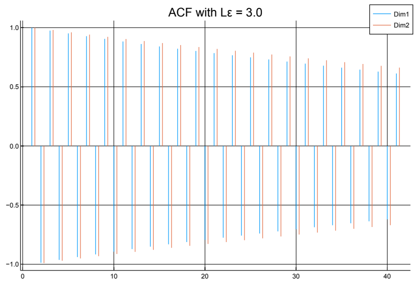


(c)

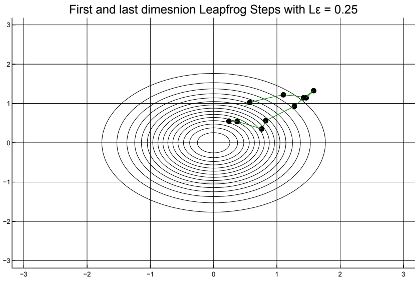


(d)

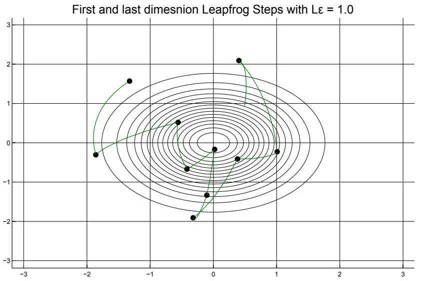


(e)

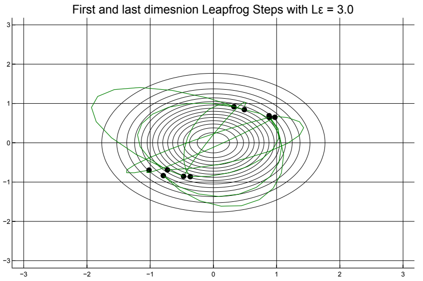


(f)

Figure S1: Tuning of HMC on a Isotropic Bivariate Normal distribution. Autocorrelation function (first line) and first 10 trajectories (second line) of the chains obtained with a small (a and d), appropriate (b and e) and large (c and f) total integration time $L\varepsilon$.

# S2 ESS by batch means

To assess the difference in efficiency between HMC and the Automatic Zig Zag, MCMCs with the two algorithms are run until a pre-defined budget is reached. The ESS of the resulting sample is then computed using the method of batch means. This is illustrated below for continuous-time samples, while for discrete-time samples we use the method described in Gilks, Richardson, and Spiegelhalter, 1995.

## S2.1 Continuous time samples

Bierkens, Fearnhead, and Roberts, 2019 proposes a method to compute the ESS of a function $h(x)$ given a continuous-time sample from a Markov chain. In this section, we assume that the function of interest is just the selection of the $i$th component of location vector $\boldsymbol{x}$, i.e. $h(\boldsymbol{x}, i) = x^{(i)}$, effectively measuring the efficiency of estimating dimension-specific means. To allow a lighter notation, we assume below that we are considering a univariate target distribution, hence we drop the index $i$, and illustrate the computation of the ESS.

A sampled continuous time MCMC in the time interval $[0, \tau]$ is stored through its $K$

skeleton points (plus one initial point $x_0, v_0, t_0 = 0$):

$$\begin{aligned} \underline{t} &= (t_0, t_1, \dots, t_k, \dots, t_K)' \\ \underline{v} &= (v_0, v_1, \dots, v_k, \dots, v_K)' \\ \underline{x} &= (x_0, x_1, \dots, x_k, \dots, x_K)' \end{aligned} \tag{1}$$

The first moment for the whole chain can be estimated as follows:

$$\begin{aligned} \widehat{M}(x) &= \frac{1}{\tau}\int_0^\tau X(s)ds \\ &= \frac{1}{t_K}\sum_{k=1}^{K}\int_{t_{k-1}}^{t_k} x_{k-1} + v_{k-1}(s - t_{k-1})ds \\ &= \frac{1}{t_K}\sum_{k=1}^{K}\frac{1}{2}\left\{(t_k - t_{k-1})\left[v_{k-1}(t_k - t_{k-1} + 2x_{k-1})\right]\right\} \end{aligned} \tag{2}$$

An estimator of the variance is:

$$\begin{aligned} \widehat{Var}(x) &= \frac{1}{\tau}\int_0^\tau [X(s)]^2\,ds - \left[\widehat{M}(x)\right]^2 \\ &= \frac{1}{t_K}\sum_{k=1}^{K}\int_{t_{k-1}}^{t_k}\left[x_{k-1} + v_{k-1}(s - t_{k-1})\right]^2 ds - \left[\widehat{M}(x)\right]^2 \\ &= \frac{1}{t_K}\sum_{k=1}^{K}\frac{\left[v_{k-1}(t_k - t_{k-1} + x_{k-1})^3\right]^3 - (x_{k-1})^3}{3v_{k-1}} - \left[\widehat{M}(x)\right]^2 \end{aligned} \tag{3}$$

To compute batch means, the interval $[0, \tau]$ must be divided in $B$ intervals of equal length $\left[(i-1)\frac{\tau}{B}; i\frac{\tau}{B}\right)$ for $i = 1, \dots B$. Let $k_l^i$ and $k_u^i$ be, respectively, the index of the lowest and uppermost skeleton points contained in $\left[(i-1)\frac{\tau}{B}; i\frac{\tau}{B}\right)$ for each interval $i = 1, \dots, B$. The first moment of batch $i$ can be computed as follows.

$$\begin{aligned} y_i =& \sqrt{\frac{B}{\tau}}\int_{\frac{i-1}{B}\tau}^{\frac{i}{B}\tau} X(s)ds \\ =& \sqrt{\frac{B}{\tau}}\,\{\int_{\frac{i-1}{B}\tau}^{t_{k_l^i}} x_{k_l^i-1} + v_{k_l^i-1}\left(s - t_{k_l^i-1}\right)ds + \int_{t_{k_l^i}}^{t_{k_l^i+1}} x_{k_l^i} + v_{k_l^i}\left(s - t_{k_l^i}\right)ds + \\ &+ \int_{t_{k_l^i+1}}^{t_{k_l^i+2}} x_{k_l^i+1} + v_{k_l^i+1}\left(s - t_{k_l^i+1}\right)ds + \dots + \\ &+ \int_{t_{k_u^i-1}}^{t_{k_u^i}} x_{k_u^i-1} + v_{k_u^i-1}\left(s - t_{k_u^i-1}\right)ds + \int_{t_{k_u^i}}^{\frac{i}{B}\tau} x_{k_u^i} + v_{k_u^i}\left(s - t_{k_u^i}\right)ds\ \} \end{aligned} \tag{4}$$

where $\int_a^b x + v(s - t_0)ds = \frac{1}{2}(a - b)\left[v(a + b - 2t_0) + 2x\right]$.

The variance of the batch means can be then estimated by:

$$\widehat{\sigma_x^2} = \frac{1}{B-1}\sum_{i=1}^{B}(Y_i - \overline{Y}) \qquad \text{with} \qquad \overline{Y} = \frac{1}{B}\sum_{i-1}^{B} Y_i \tag{5}$$

The ESS of the continuous time sample can then be estimated by;

$$\widehat{ESS}^{\text{ZZ}} = \tau \frac{\widehat{Var}(x)}{\widehat{\sigma_x^2}} \tag{6}$$

### S2.2 Selection of batch size

The value taken by the ESS estimated via batch means is highly dependent on the number of batches (hence batch size) chosen, both for continuous-time and discrete-time MCMCs. When the number of batches $B$ is too small or too large, the ESS will be over-estimated. To allow for a fair comparison between the two methods we select the $B$ that minimizes the average ESS in the slowing-moving dimension (i.e. the dimension with lowest ESS).

Figure S2 shows how is this done in the setting of an Automatic Zig-Zag sampler on a bivariate Normal distribution. 100 chains are run on the target and their skeleton is saved. Five potential values for $B$ are selected: $B = 10, 100, 500, 1000, 2000$ and the ESS is computed at these different values. The lowest ESS for both dimensions is reached for $B = 100$, this is then used to obtain the results of the performance comparison.

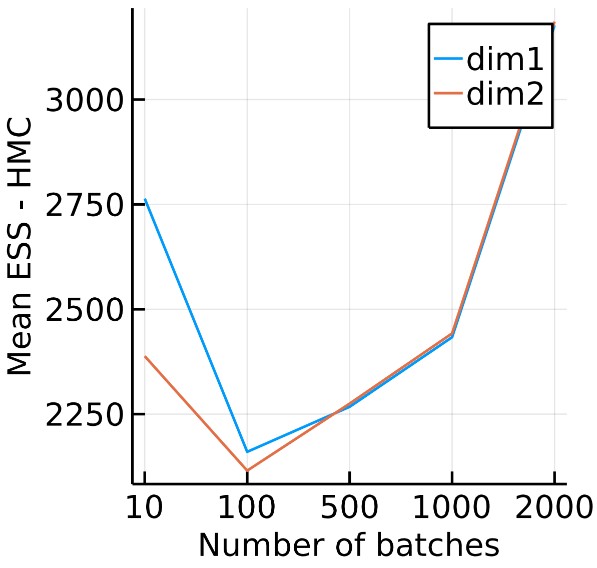


Figure S2: Choice of the batch size $B$.

# S3 Supplementary results of simulation study for the performance comparison

The density functions of the bivariate distributions used for the performance evaluation in Section 4 of the main text are plotted in Figure S3. These are: an isotropic Gaussian distribution (`IsoG2`); a bivariate Gaussian distribution where the two component had same scale and high correlation $\rho = 0.9$ (`CorG2`); a bivariate Gaussian distribution with independent component with very different scales $\sigma_1^2 = 1, \sigma_2^2 = 100$ (`DscG2`); an heavy-tailed distribution (`HT2`); a light-tailed distribution (`LT2`); and on a bimodal distribution, a mixture of Gaussians (`BimodG2`).

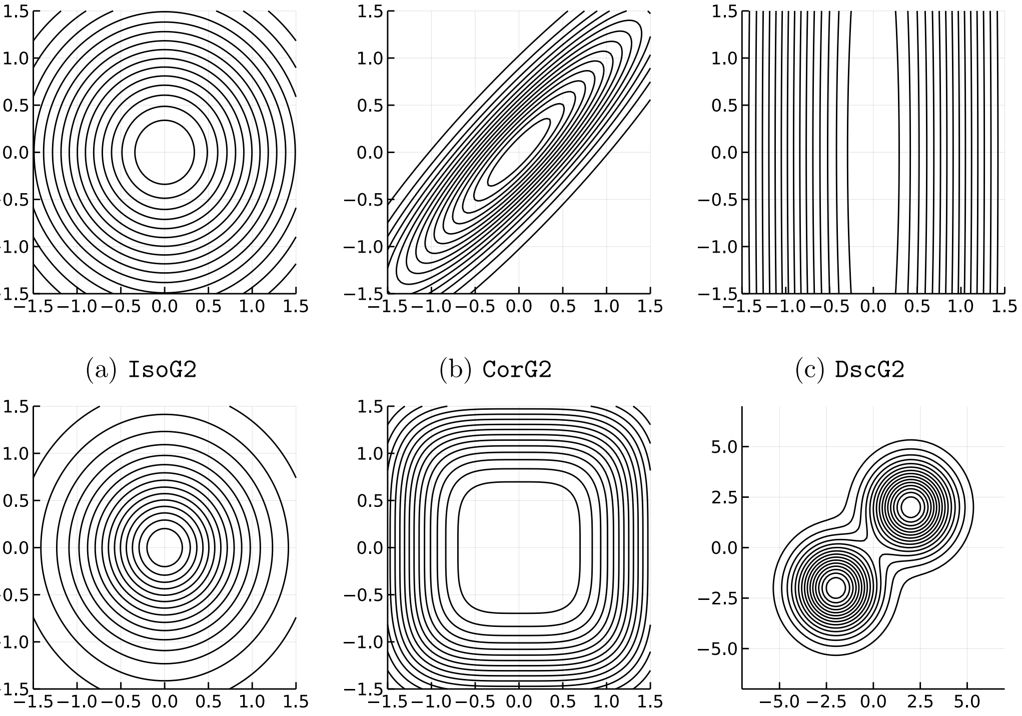

(a) `IsoG2` (b) `CorG2` (c) `DscG2`

(d) `HT2` (e) `LT2` (f) `BimodG2`

Figure S3: Contour plots of the probability density function of the target distributions used for the performance evaluation of the Automatic Zig-Zag sampler.

## S3.1 Isotropic bivariate normal

The target distribution is a bivariate Gaussian with independent standard components:

$$\boldsymbol{X} \sim \mathcal{N}_d \left( \begin{bmatrix} 0 \\ 0 \end{bmatrix}, \begin{bmatrix} 1 & 0 \\ 0 & 1 \end{bmatrix} \right).$$

The parameter $t_{\text{MAX}}$ was tuned and set to 2.5, which leads to the most efficient algorithm (as in Figure S4).

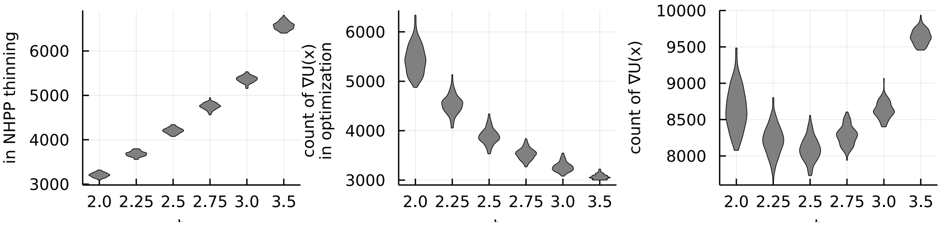


Figure S4: Number of gradient evaluations in the simulation-steps of the non-homogeneous Poisson process (NHPP) via thinning (left), in the optimization steps (centre), and total number of gradient evaluations (right) form 100 samples of 1000 skeleton points.

Table S1 and Figure S5 provide a comparison between HMC and Automatic Zig-Zag sampling in terms of dimension-specific ESS obtained on 100 simulations with a budget of 20,000 gradient evaluations.

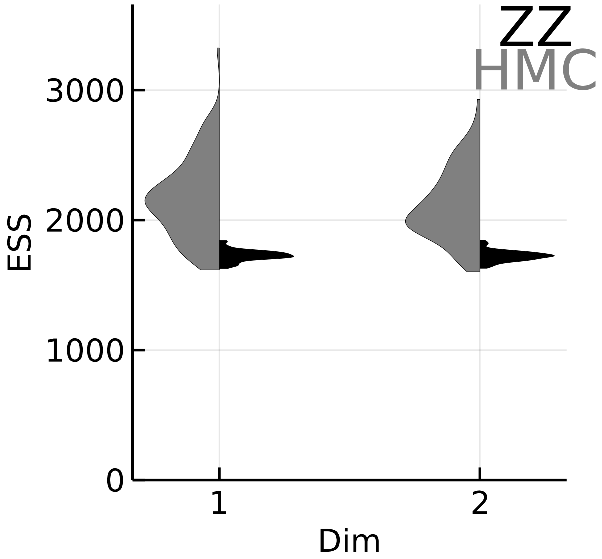


Figure S5: Violin plot of the ESS of each dimension obtained on 100 simulated chains of HMC and Automatic Zig-Zag.

| | Dim 1 | | Dim 2 | |
|---|---|---|---|---|
| | Automatic ZZ | HMC | Automatic ZZ | HMC |
| Mean | 1727.45 | 2160.09 | 1723.85 | 2115.29 |
| Minimum | 1625.31 | 1614.61 | 1628.21 | 1605.17 |
| $1^{st}$ quartile | 1706.1 | 1949.85 | 1695.74 | 1934.59 |
| Median | 1728.51 | 2142.63 | 1723.27 | 2049.19 |
| $3^{rd}$ quartile | 1751.06 | 2326.49 | 1747.58 | 2307.77 |
| Maximum | 1845.0 | 3326.11 | 1845.6 | 2928.35 |

Table S1: Summary statistics of the ESS obtained with the Automatic Zig-Zag algorithm and HMC algorithm given the pre-specified budget.

HMC and Automatic Zig-Zag were equally robust with chains starting form the mode (Figures S6a and S6c) and from the tails (Figures S6b and S6d) rapidly converging to the correct distribution.

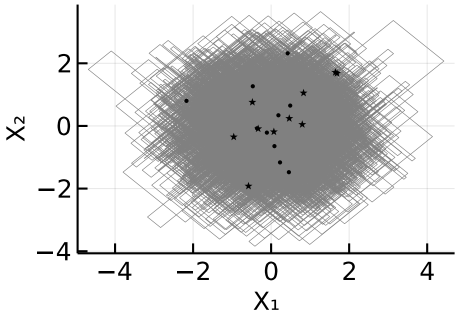


(a) Automatic Zig-Zag starting from the mode

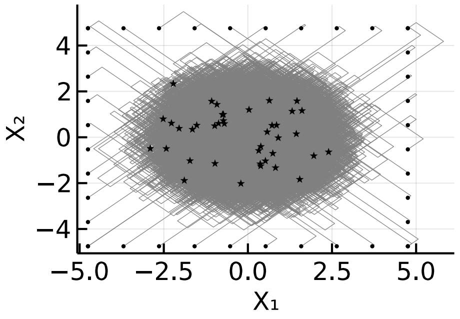


(b) Automatic Zig-Zag starting from the tail

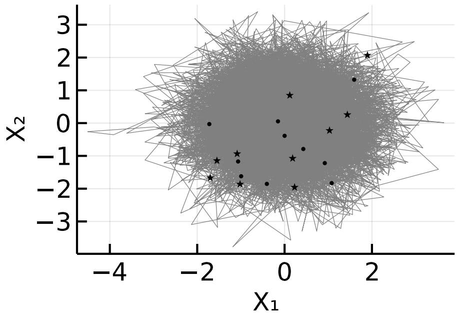


(c) HMC starting from the mode

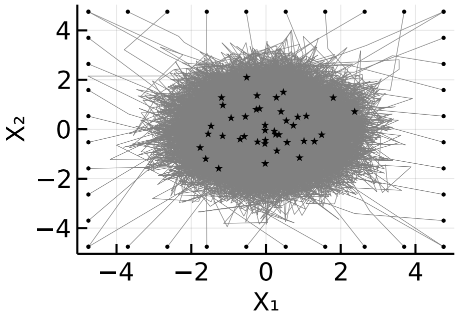


(d) HMC starting from the tail

Figure S6: Robustness of the two algorithms.

### S3.2 Correlated bivariate normal

The target distribution is a bivariate Gaussian with independent standard components:

$$\boldsymbol{X} \sim \mathcal{N}_d \left( \begin{bmatrix} 0 \\ 0 \end{bmatrix}, \begin{bmatrix} 1 & 0.90 \\ 0.90 & 1 \end{bmatrix} \right).$$

The parameter $t_{\text{MAX}}$ was tuned and set to 1.0, which leads to the most efficient algorithm (as in Figure S7).

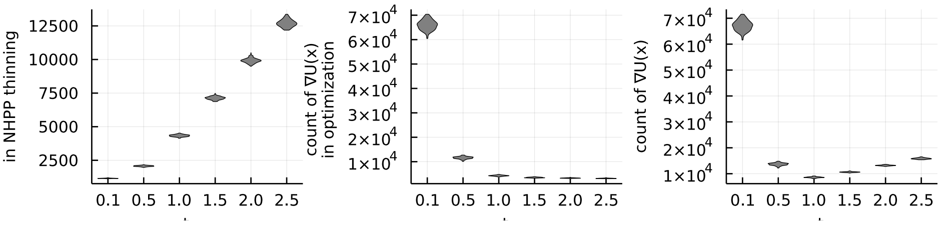


Figure S7: Number of gradient evaluations in the simulation-steps of the NHPP via thinning (left), in the optimization steps (centre), and total number of gradient evaluations (right) form 100 samples of 1000 skeleton points.

Table S2 and Figure S8 provide a comparison between HMC and Automatic Zig-Zag sampling in terms of dimension-specific ESS obtained on 100 simulations with a budget of 20,000 gradient evaluations.

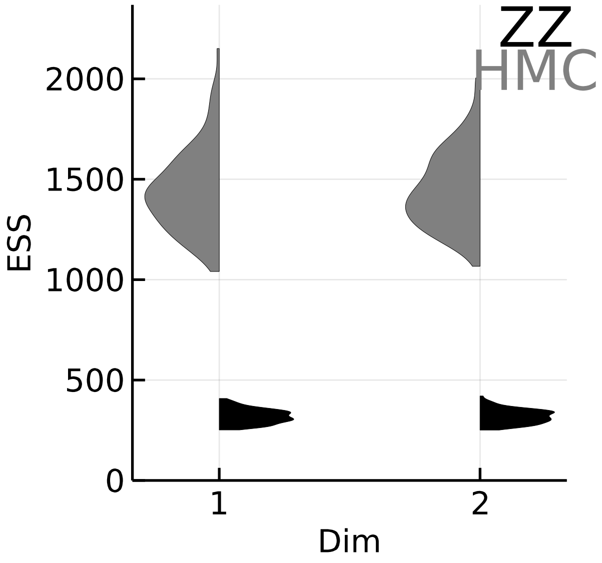


Figure S8: Violin plot of the ESS of each dimension obtained on 100 simulated chains of HMC and Automatic Zig-Zag.

| | Dim 1 | | Dim 2 | |
|---|---|---|---|---|
| | Automatic ZZ | HMC | Automatic ZZ | HMC |
| Mean | 319.11 | 1442.31 | 318.26 | 1447.49 |
| Minimum | 250.73 | 1038.47 | 249.92 | 1061.06 |
| $1^{st}$ quartile | 292.96 | 1303.12 | 291.48 | 1294.5 |
| Median | 317.76 | 1426.43 | 316.94 | 1418.7 |
| $3^{rd}$ quartile | 344.36 | 1570.59 | 344.85 | 1585.34 |
| Maximum | 409.13 | 2153.08 | 421.89 | 2009.99 |

Table S2: Summary statistics of the ESS obtained with the Automatic Zig-Zag algorithm and HMC algorithm given the pre-specified budget.

HMC and Automatic Zig-Zag were equally robust with chains starting form the mode (Figures S9a and S9c) and from the tails (Figures S9b and S9d) rapidly converging to the correct distribution.

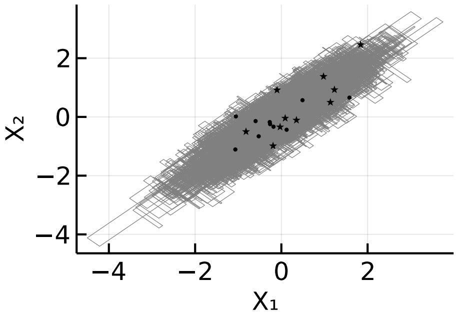


(a) Automatic Zig-Zag starting from the mode

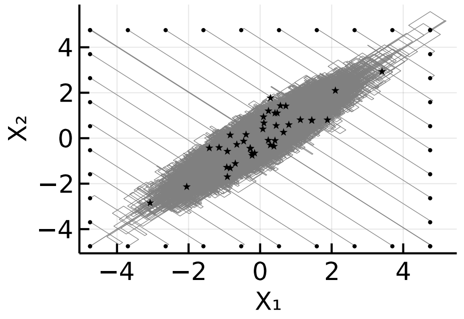


(b) Automatic Zig-Zag starting from the tail

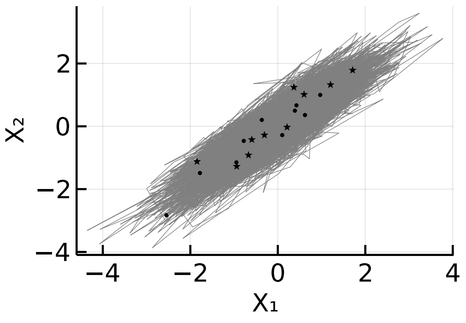


(c) HMC starting from the mode

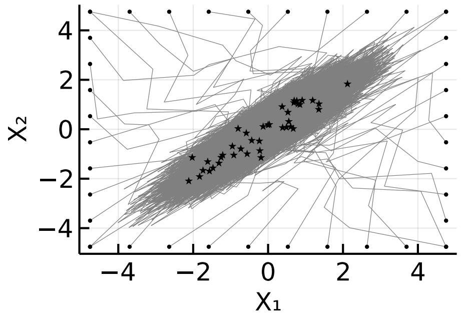


(d) HMC starting from the tail

Figure S9: Robustness of the two algorithms.

### S3.3 Bivariate normal on different scales

The target distribution is a bivariate Gaussian with independent standard components:

$$\boldsymbol{X} \sim \mathcal{N}_d\left(\begin{bmatrix}0\\0\end{bmatrix}, \begin{bmatrix}1 & 0\\0 & 100\end{bmatrix}\right).$$

The parameter $t_{\mathrm{MAX}}$ was tuned and set to 4, which leads to the most efficient algorithm (as in Figure S10).

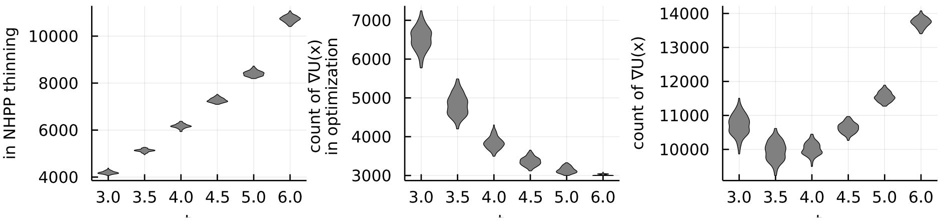


Figure S10: Number of gradient evaluations in the simulation-steps of the NHPP via thinning (left), in the optimization steps (centre), and total number of gradient evaluations (right) form 100 samples of 1000 skeleton points.

Table S3 and Figure S11 provide a comparison between HMC and Automatic Zig-Zag sampling in terms of dimension-specific ESS obtained on 100 simulations with a budget of 20,000 gradient evaluations.

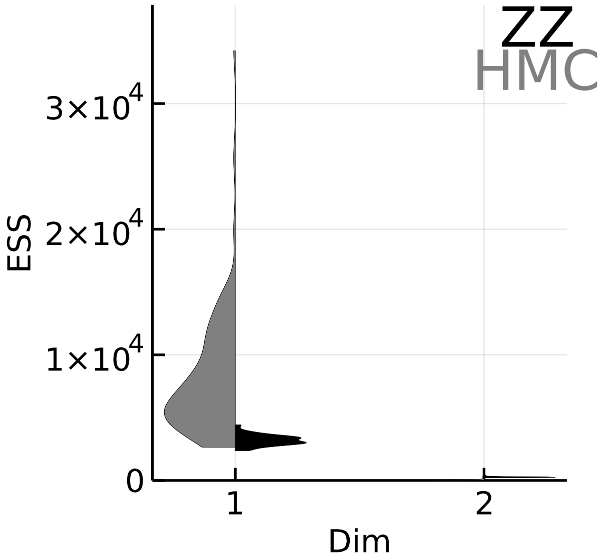


Figure S11: Violin plot of the ESS of each dimension obtained on 100 simulated chains of HMC and Automatic Zig-Zag.

| | Dim 1 | | Dim 2 | |
|---|---|---|---|---|
| | Automatic ZZ | HMC | Automatic ZZ | HMC |
| Mean | 3205.43 | 8019.13 | 265.46 | 50.59 |
| Minimum | 2360.08 | 2434.81 | 214.19 | 21.14 |
| $1^{st}$ quartile | 2927.41 | 5066.06 | 239.41 | 32.64 |
| Median | 3174.3 | 6770.05 | 261.5 | 43.56 |
| $3^{rd}$ quartile | 3458.34 | 10359.31 | 283.52 | 57.17 |
| Maximum | 4441.71 | 34413.62 | 405.3 | 288.71 |

Table S3: Summary statistics of the ESS obtained with the Automatic Zig-Zag algorithm and HMC algorithm given the pre-specified budget.

HMC and Automatic Zig-Zag were equally robust with chains starting form the mode (Figures S12a and S12c) and from the tails (Figures S12b and S12d) rapidly converging to the correct distribution.

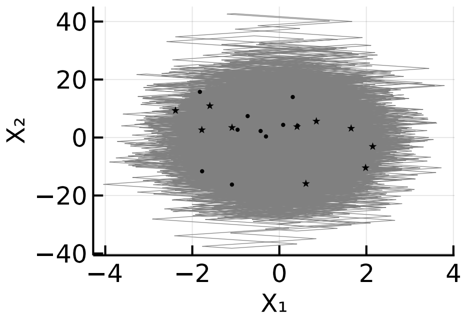


(a) Automatic Zig-Zag starting from the mode

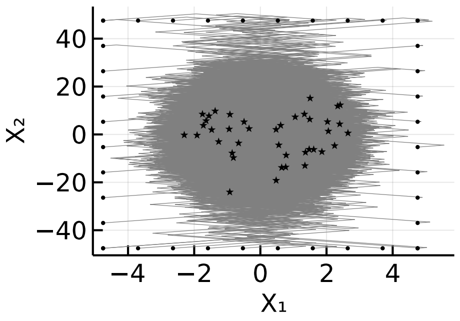


(b) Automatic Zig-Zag starting from the tail

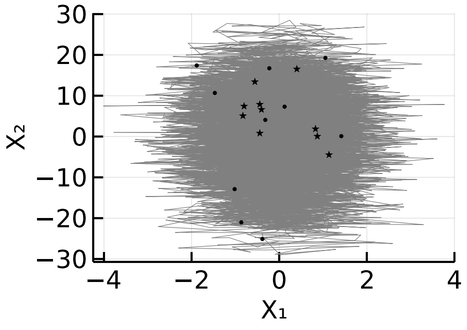


(c) HMC starting from the mode

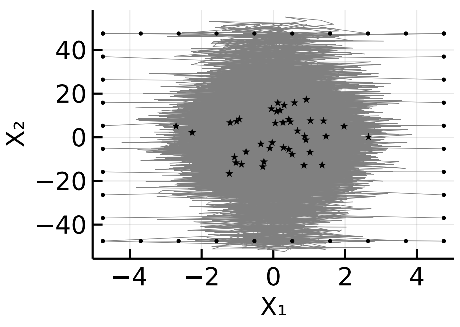


(d) HMC starting from the tail

Figure S12: Robustness of the two algorithms.

## S3.4 Heavy-tailed bivariate distribution

The target distribution is a bivariate Student-T with two degrees of freedom:

$$\boldsymbol{X} \sim \mathcal{T}_2 (\nu = 2) .$$

The parameter $t_{\mathrm{MAX}}$ was tuned and set to 5, which leads to the most efficient algorithm (as in Figure S13).

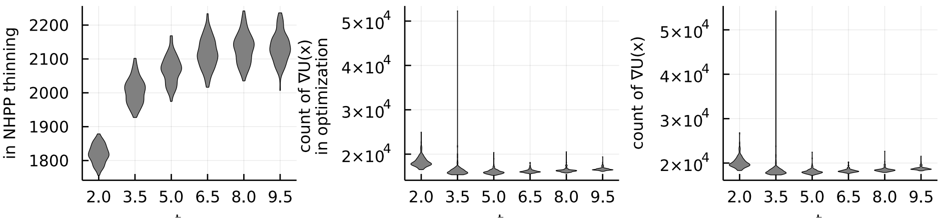


Figure S13: Number of gradient evaluations in the simulation-steps of the NHPP via thinning (left), in the optimization steps (centre), and total number of gradient evaluations (right) form 100 samples of 1000 skeleton points.

Table S4 and Figure S14 provide a comparison between HMC and Automatic Zig-Zag sampling in terms of dimension-specific ESS obtained on 100 simulations with a budget of 20,000 gradient evaluations.

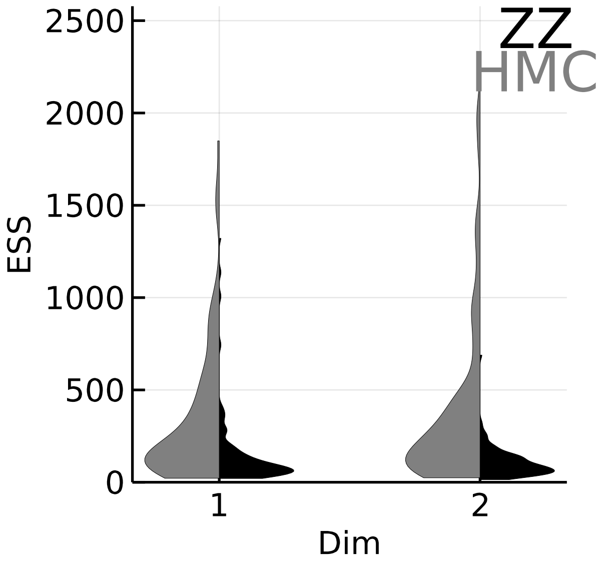


Figure S14: Violin plot of the ESS of each dimension obtained on 100 simulated chains of HMC and Automatic Zig-Zag.

| | Dim 1 | | Dim 2 | |
|---|---|---|---|---|
| | Automatic ZZ | HMC | Automatic ZZ | HMC |
| Mean | 148.82 | 343.38 | 106.94 | 389.21 |
| Minimum | 14.16 | 13.86 | 10.64 | 12.53 |
| $1^{st}$ quartile | 52.83 | 101.36 | 55.19 | 87.9 |
| Median | 86.25 | 182.12 | 84.79 | 220.07 |
| $3^{rd}$ quartile | 146.52 | 480.48 | 136.25 | 439.3 |
| Maximum | 1327.56 | 1856.75 | 692.02 | 2343.75 |

Table S4: Summary statistics of the ESS obtained with the Automatic Zig-Zag algorithm and HMC algorithm given the pre-specified budget.

HMC is less robust than Automatic Zig-Zag with chains starting form the mode properly exploring the tails, (Figures S15a and S15c), however, when started from the tails (Figures S15b and S15d) HMC chains do not converge to the mode of the distribution as fast as Automatic Zig-Zag.

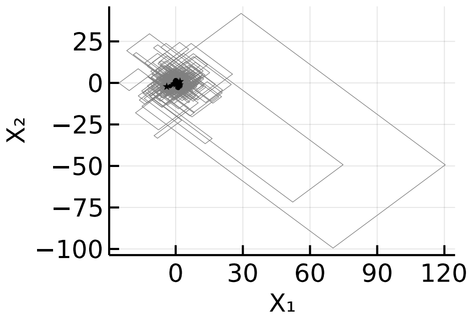


(a) Automatic Zig-Zag starting from the mode

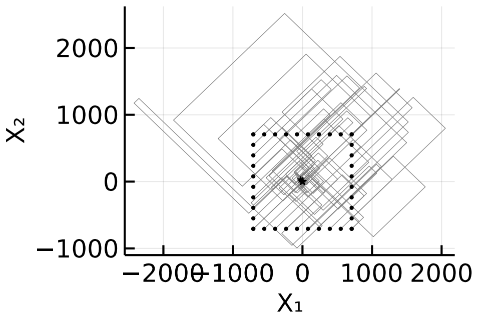


(b) Automatic Zig-Zag starting from the tail

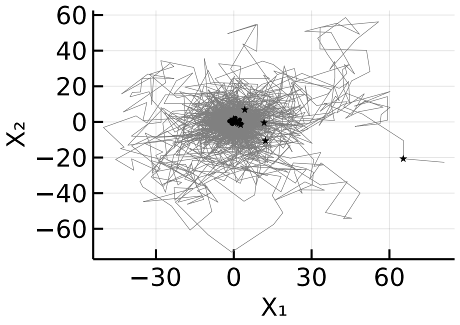


(c) HMC starting from the mode

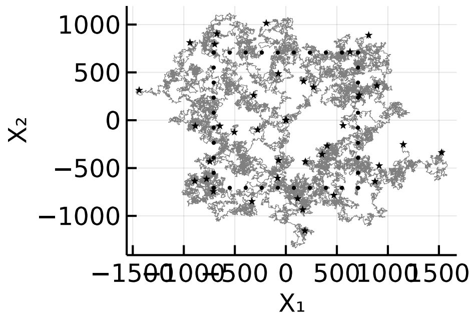


(d) HMC starting from the tail

Figure S15: Robustness of the two algorithms.

## S3.5 Light-tailed bivariate distribution

The target distribution is a bivariate distribution with density:

$$\pi(\boldsymbol{x}) \propto e^{x_1^4/4+x_2^4/4}$$

The parameter $t_{\mathrm{MAX}}$ was tuned and set to 1.5, which leads to the most efficient algorithm (as in Figure S16).

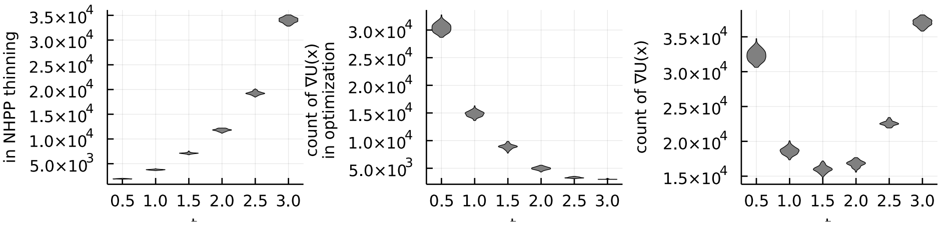


Figure S16: Number of gradient evaluations in the simulation-steps of the NHPP via thinning (left), in the optimization steps (centre), and total number of gradient evaluations (right) form 100 samples of 1000 skeleton points.

Table S5 and Figure S17 provide a comparison between HMC and Automatic Zig-Zag sampling in terms of dimension-specific ESS obtained on 100 simulations with a budget of 20,000 gradient evaluations.

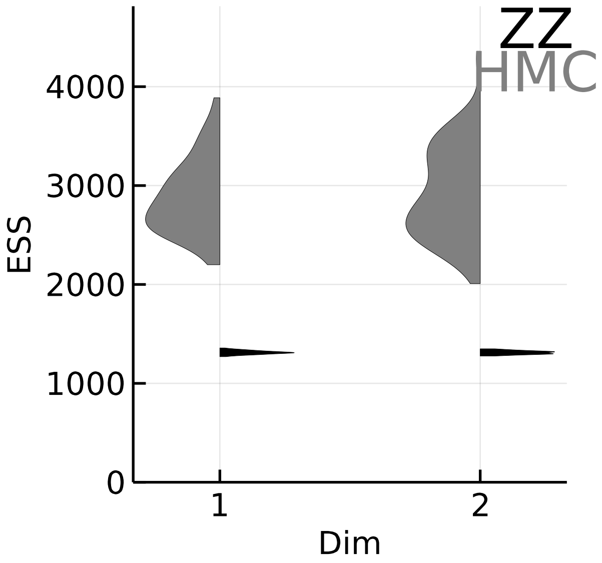


Figure S17: Violin plot of the ESS of each dimension obtained on 100 simulated chains of HMC and Automatic Zig-Zag.

| | Dim 1 | | Dim 2 | |
|---|---|---|---|---|
| | Automatic ZZ | HMC | Automatic ZZ | HMC |
| Mean | 1312.2 | 2881.56 | 1311.86 | 2925.94 |
| Minimum | 1269.57 | 2194.25 | 1276.23 | 1991.27 |
| $1^{st}$ quartile | 1301.02 | 2597.08 | 1297.71 | 2563.12 |
| Median | 1311.07 | 2819.88 | 1311.95 | 2844.82 |
| $3^{rd}$ quartile | 1325.24 | 3118.04 | 1323.84 | 3312.2 |
| Maximum | 1358.18 | 3892.99 | 1349.61 | 4375.72 |

Table S5: Summary statistics of the ESS obtained with the Automatic Zig-Zag algorithm and HMC algorithm given the pre-specified budget.

HMC performs equally well to Automatic Zig-Zag with chains starting form the mode (Figures S18a and S18c). When started from the tails, instead, HMC does not move from its initial points (Figure S18b) while Automatic Zig-Zag rapidly converges to the mode of the distribution (Figure S18d).

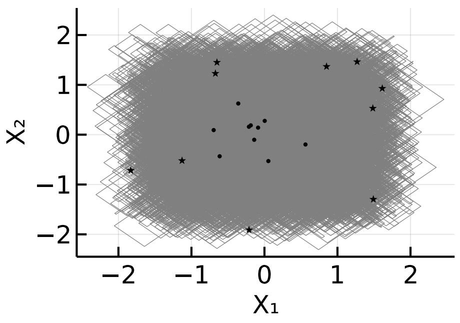


(a) Automatic Zig-Zag starting from the mode

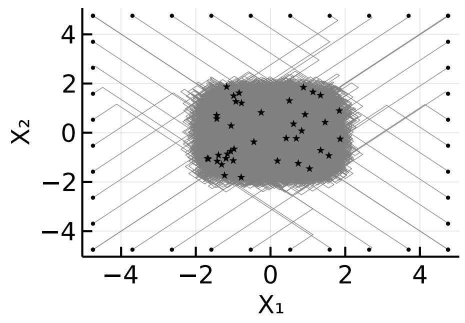


(b) Automatic Zig-Zag starting from the tail

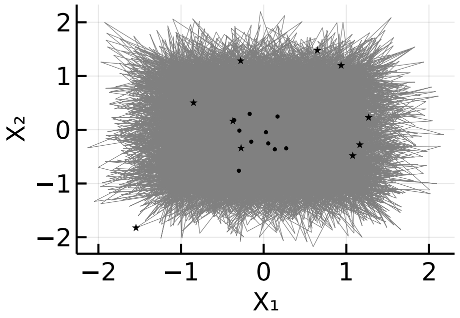


(c) HMC starting from the mode

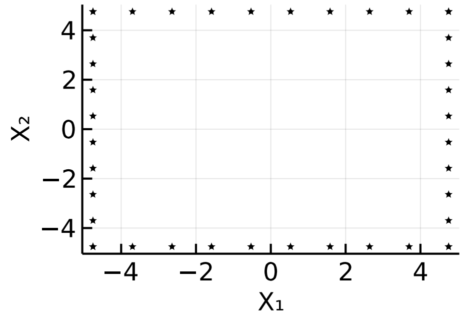


(d) HMC starting from the tail

Figure S18: Robustness of the two algorithms.

### S3.6 Bimodal bivariate distribution: Mixture of normals

The target distribution is a bivariate distribution with density:

$$\boldsymbol{X_1} \sim \mathcal{N}_d\left(\begin{bmatrix}-2\\-2\end{bmatrix}, \begin{bmatrix}1 & 0\\0 & 1\end{bmatrix}\right)$$

$$\boldsymbol{X_2} \sim \mathcal{N}_d\left(\begin{bmatrix}+2\\+2\end{bmatrix}, \begin{bmatrix}1 & 0\\0 & 1\end{bmatrix}\right)$$

$$f_{\boldsymbol{X}}(\boldsymbol{x}) = 0.5 f_{\boldsymbol{X_1}}(\boldsymbol{x}) + 0.5 f_{\boldsymbol{X_2}}(\boldsymbol{x})$$

The parameter $t_{\text{MAX}}$ was tuned and set to 4, which leads to the most efficient algorithm (as in Figure S19).

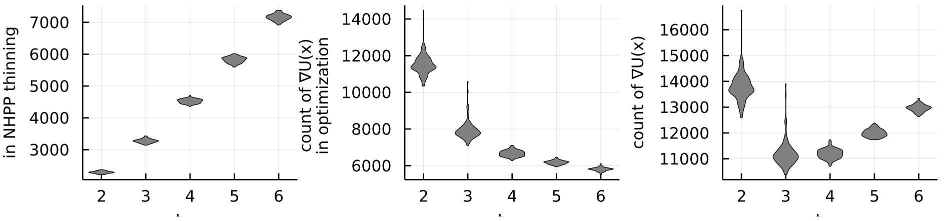


Figure S19: Number of gradient evaluations in the simulation-steps of the NHPP via thinning (left), in the optimization steps (centre), and total number of gradient evaluations (right) form 100 samples of 1000 skeleton points.

Table S6 and Figure S20 provide a comparison between HMC and Automatic Zig-Zag sampling in terms of dimension-specific ESS obtained on 100 simulations with a budget of 20,000 gradient evaluations.

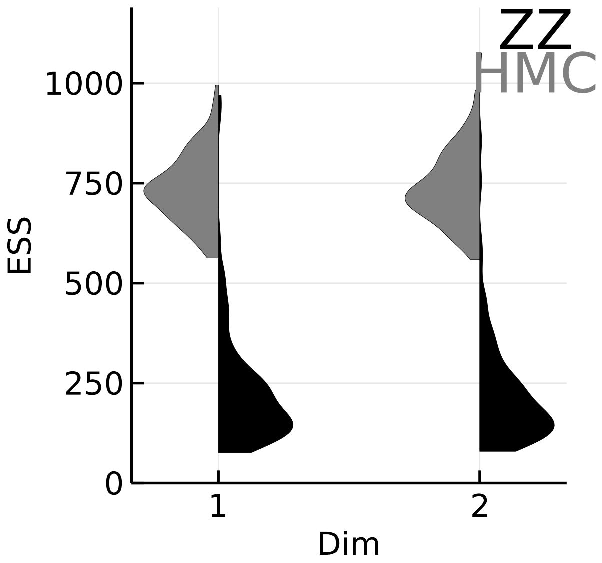


Figure S20: Violin plot of the ESS of each dimension obtained on 100 simulated chains of HMC and Automatic Zig-Zag.

| | Dim 1 | | Dim 2 | |
|---|---|---|---|---|
| | Automatic ZZ | HMC | Automatic ZZ | HMC |
| Mean | 231.54 | 737.14 | 230.9 | 737.21 |
| Minimum | 74.39 | 560.42 | 73.16 | 557.11 |
| $1^{st}$ quartile | 139.26 | 678.18 | 137.55 | 682.95 |
| Median | 189.89 | 734.18 | 184.6 | 727.37 |
| $3^{rd}$ quartile | 270.53 | 790.54 | 263.97 | 798.87 |
| Maximum | 972.13 | 997.8 | 1081.35 | 983.84 |

Table S6: Summary statistics of the ESS obtained with the Automatic Zig-Zag algorithm and HMC algorithm given the pre-specified budget.

HMC performs equally well to Automatic Zig-Zag with chains starting form the mode (Figures S21a and S18c) and from the tail (Figure S21b and S21d).

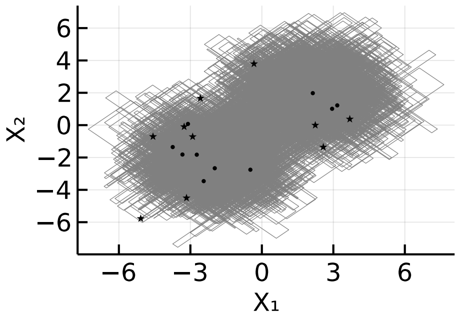

(a) Automatic Zig-Zag starting from the mode

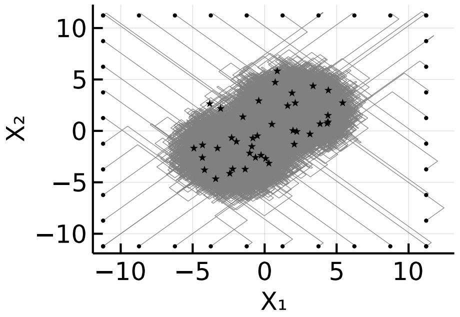

(b) Automatic Zig-Zag starting from the tail

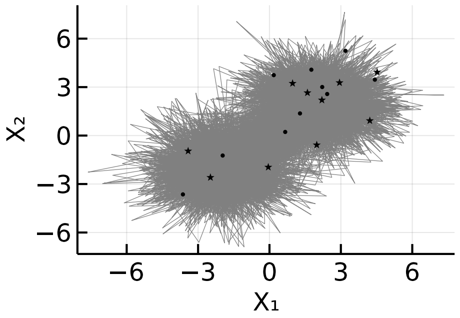

(c) HMC starting from the mode

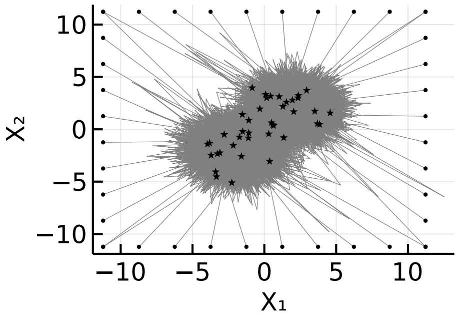

(d) HMC starting from the tail

Figure S21: Robustness of the two algorithms.

# S4 Supplementary results of the real-data analyses

## S4.1 A textbook example

The parameter $t_{\mathrm{MAX}}$ was tuned and set to 0.02, which leads to the most efficient algorithm (as in Figure S22).

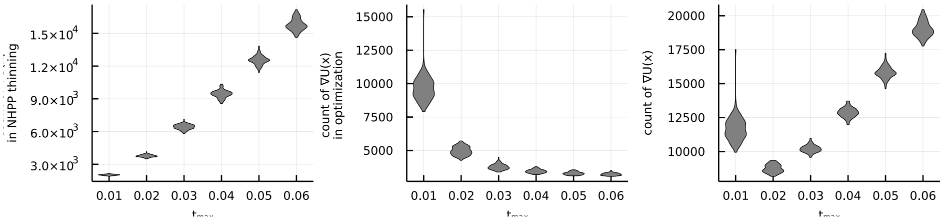


Figure S22: Number of gradient evaluations in the simulation-steps of the NHPP via thinning (left), in the optimization steps (centre), and total number of gradient evaluations (right) form 100 samples of 1000 skeleton points.

Figure S23 provides a comparison between HMC and Automatic Zig-Zag sampling in terms of dimension-specific ESS obtained on 100 simulations with a budget of 200,000 gradient evaluations.

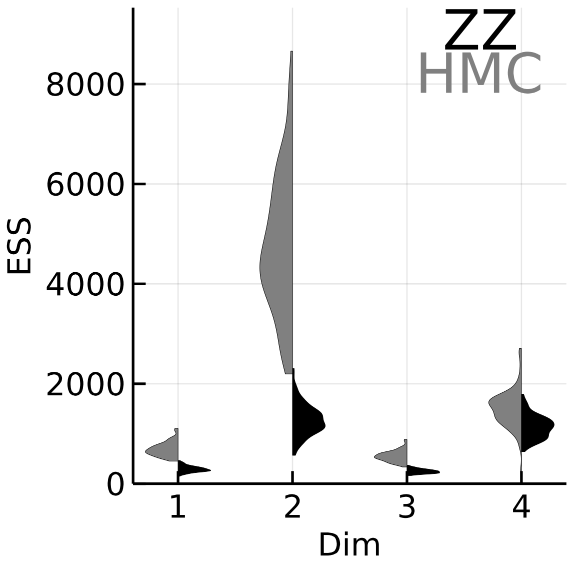


Figure S23: Violin plot of the ESS of each dimension obtained on 100 simulated chains of HMC and Automatic Zig-Zag.

### S4.2 Parametric survival model

The parameter $t_{\text{MAX}}$ was tuned and set to 0.1, which leads to the most efficient algorithm (as in Figure S24).

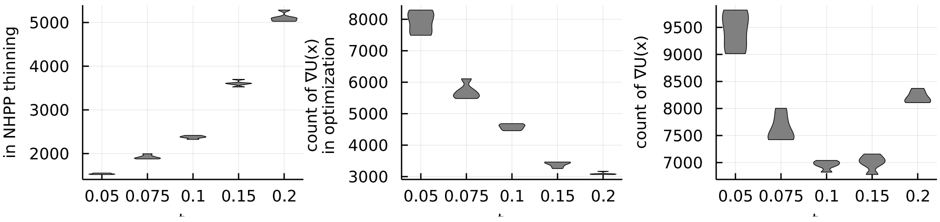


Figure S24: Number of gradient evaluations in the simulation-steps of the NHPP via thinning (left), in the optimization steps (centre), and total number of gradient evaluations (right) form 100 samples of 1000 skeleton points.

HMC performs equally well to Automatic Zig-Zag with chains starting form the mode (Figures S25a and S25c) but struggles to reach areas of higher mass when the chains are initiated in the tail (Figure S25d).

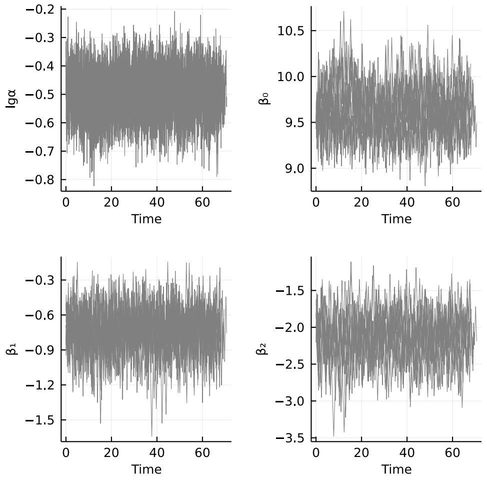


(a) Automatic Zig-Zag starting from the mode

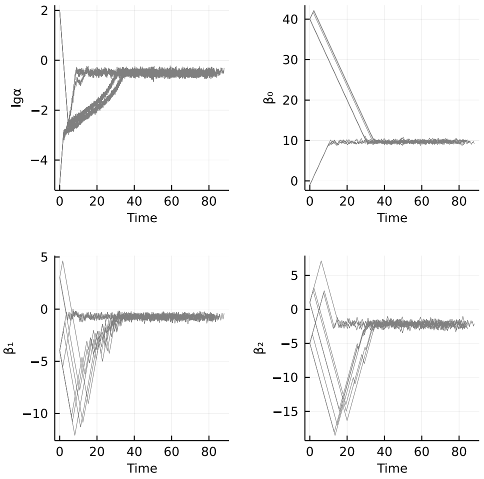


(b) Automatic Zig-Zag starting from the tail

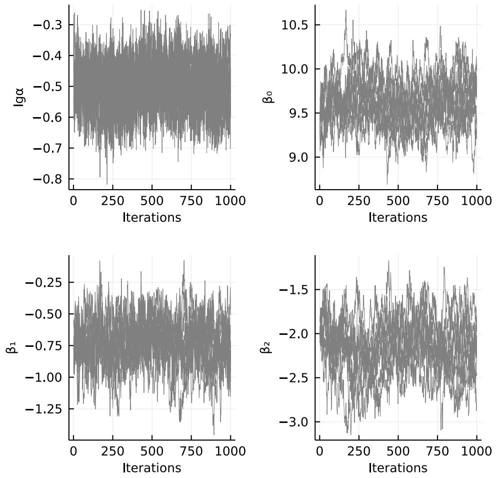


(c) HMC starting from the mode

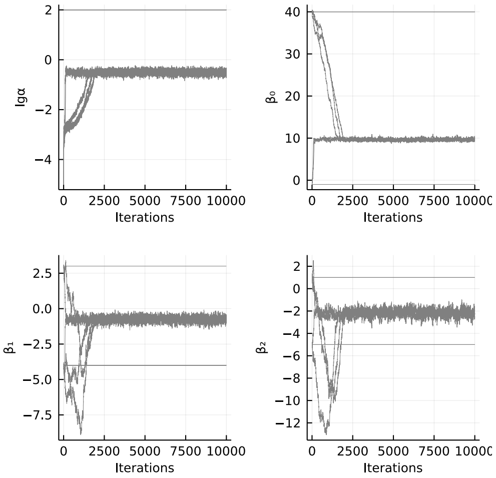


(d) HMC starting from the tail

Figure S25: Robustness of the two algorithms.

# S5 Application of extreme value theory and parameter tuning

There are two approaches to estimate the distribution of a maximum: blocked maximum and threshold-exceedance. The first consists of dividing the data in blocks and considering the highest value of each block as a maximum; the latter instead sets a threshold above which a value is considered to be maximum and then retains the differences between these maxima and the threshold. The threshold-exceedance method uses all the

information in the tail, while the blocked maximum is likely to discard high values if more then one happens in the same block. For this reason we estimate $\widehat{c}$, the population local upper bound, using the latter, also known as peak over threshold (POT).

### S5.1 Threshold-exceedance

This section introduces the POT approach to the modelling of extreme values and reports some key results from Wadsworth, 2016.

Assume to have a sequence of independent and identically distributed (iid) random variables (rvs) $X_1, X_2, \ldots, X_n \sim F$. Given a threshold $u$ consider the set $\mathcal{E}$ of the indexes of the rvs that exceed $u$; then the appropriately scaled excesses $X_i - u$ for $i \in \mathcal{E}$, converge to the Generalised Pareto Distribution (GPD), with cumulative distribution function:

$$H(x) = 1 - \max\{[1 + \xi x/\sigma], 0\}^{-1/\xi} \qquad \sigma > 0, \xi \in \mathbb{R} \tag{7}$$

as $u \to x^F$, the upper endpoint of the support. If GPD approximation holds, then the normalised maxima $M_n = \max\{X_1, \ldots X_n\}$ converge to a Generalised Extreme Value (GEV) distribution with the shape parameter $\xi$ being the same for both GEV and GPD. However, if all the data $X_i$s are available, the POT approach should be more efficient as more information is retained.

### S5.2 Choice of threshold and estimation of return values

The threshold $u$ needs to be chosen so that it would be large enough to guarantee the convergence to a GPD and small enough so that the number of observations above the threshold are sufficient to infer the parameter of the distribution.

In our case we choose $u$ to be the 95% quantile of the samples $x_1, x_2, \ldots, x_n$. In our context, $n$ is the number of selected rate-specific bounds and can be chosen arbitrary. We will then chose it so that the number of observations above the threshold is equal or larger than 30, i.e. $n \geq 600$.

The parameters $\xi$ and $\sigma$ can be estimated via maximum likelihood with the use of packages that run numeric optimization algorithms, as a closed-form maximul likelihood estimator (MLE) does not exist.

Given estimates $\widehat{\xi}$ and $\widehat{\sigma}$, the $m$ return value, i.e. the high quantile for which the probability that the maximum exceeds this quantile is $1/m$ can be obtained using (7).

## References


Bierkens, J., P. Fearnhead, and G. Roberts (2019). "The zig-zag process and super-efficient sampling for Bayesian analysis of big data". In: *The Annals of Statistics* 47.3, pp. 1288–1320.

Gilks, W. R., S. Richardson, and D. Spiegelhalter (1995). *Markov chain Monte Carlo in practice.* CRC press.

Neal, R. M. et al. (2011). "MCMC using Hamiltonian dynamics". In: *Handbook of Markov Chain Monte Carlo* 2.11, p. 2.

Sherlock, C., S. Urbas, and M. Ludkin (2021). “Apogee to Apogee Path Sampler”. In: *arXiv preprint arXiv:2112.08187*.

Wadsworth, J. L. (2016). “Exploiting structure of maximum likelihood estimators for extreme value threshold selection”. In: *Technometrics* 58.1, pp. 116–126.
